# Supplementary material for: KuraNet: Systems of Coupled Oscillators that Learn to Synchronize
Source: arXiv:2105.02838 ancillary file (2021-05-06)
Supplement: Supplementary file 1 [file SI.pdf]

# SUPPLEMENTARY INFORMATION FOR "KURANET: SYSTEMS OF COUPLED OSCILLATORS THAT LEARN TO SYNCHRONIZE"

## 1 Methods

All Python 3 code is available at `https://github.com/serre-lab/KuraNet`.

### 1.1 Data

For all experiments except those with images, 20,000 i.i.d. random node features were generated in advance and split into training and test sets, each with $N = 10,000$ features. For image segmentation experiments, each image was divided into three random equally-sized train and test splits and the results for the best splits are shown. Global synchrony experiments used node features comprising random intrinsic frequencies, external field strengths and delays, denoted by $\omega, b$ and $\tau$ respectively. The specific combinations of these features differed among experiments with at least one parameter obeying the degenerate distribution, $\delta(0)$: Case I used $\omega \sim U([-1, 1])$, $b \sim \delta(0)$, $\tau \sim \delta(0)$; Case II used $\omega \sim U([-1, 1])$, $b \sim U([-1, 1])$, $\tau \sim \delta(0)$; Case III used $\omega \sim U([2, 4])$, $b \sim \delta(0)$, $\tau \sim NB(.5, 15)$. During training, each node on the underlying graph on each iteration was randomly assigned a feature, $x$, from the joint distribution, $D$, on $(\omega, b, \tau)$ (assuming independence). We use superscripts to index samples from $D$ and subscripts denote a particular dimension of this sample. That is, the $i^{\text{th}}$ sample from $D$ is $x^{(i)}$ and the value of this sample in the $v^{\text{th}}$ dimension is $x_v^{(i)}$. Mixture distribution data were generated from the built-in distributions in Python's `sklearn` module.

Cluster synchrony node features were drawn either from simple mixture distributions or from nine images in the Berkeley Segmentation Data Set (BSDS, `https://www2.eecs.berkeley.edu/Research/Projects/CS/vision/grouping/resources.html`). Mixture data were again sampled from `sklearn` distributions on the plane: two interlinked spirals ("Spirals"), two interlinked crescent moons ("Moons"), two concentric circles ("Circles") as well as nine Gaussian mixture models (GMM$k$) with $k = 2, \ldots, 10$ means spaced evenly around a ring of radius 10. Each graph node was assigned a two-dimensional sample $x = (p, q)$ at each training iteration. Similarly, each node in the image segmentation setting was assigned a five-dimensional sample, $x = (p, q, I_r, I_g, I_b)$, comprising not only the integer pixel location $(p, q)$ but also the color channel intensities $(I_r, I_g, I_b)$ at that location.

We note three important values related to the size of data used in our simulations: the data set size, the mini-batch size and the dynamic batch size. The data set size, $N$, is simply the number of node features which are generated in advance for each simulation; e.g., 10,000 for the global synchrony experiments. The mini-batch size, $n$, is the number of features sampled from the data set on each training iteration. These $n$ features correspond to a Kuramoto network of $n$ nodes. Finally, the dynamic batch size, $m$, is the number of nodes updated at each time-step in the dynamics. For large $n$, we typically set $m < n$ to prevent memory overflow (see Sections 1.3, 1.5). Depending on the simulation, some of these values can be equal. For instance, during training we set $m = n$ but $n < N$. On the other hand, for the "Size" testing regime, we set $n = N$ but $m < n$.

### 1.2 Neural architecture

All experiments used the same multilayer perceptron (MLP) neural architecture but differed in the way that the raw MLP output, $A$, was transformed into couplings, $K$. The MLP structure was chosen for simplicity, and architectural parameters were all set at standard values used in the machine learning literature. For $d$-dimensional node features, we used a 3-layer MLP with a $2d$-dimensional input layer (to accommodate pairs of features) and a 1-dimensional output. The hidden layer had 100 units. The MLP was applied to all $m(m-1)$ distinct pairs of input features in

parallel, where $m \leq n$ is the dynamic batch size and $n$ is the total network size (see Sections 1.1, 1.4). We set $m = 100$ for all experiments. The outputs of the first and second layers were passed through a leaky zero-rectified (LReLU) non-linearity. These layers were also batch-normalized [1] to improve stability during learning. The fact that the architecture maps from pairs of features $(x^{(i)}, x^{(j)})$ to a single real value representing the affinity of these features makes the neural architecture similar to a "relational network" [2]. The trainable parameters, $\mu$, of the network comprise its synaptic weights and biases together with the activity means and variances stored in batch normalization layers. The architecture was implemented in `pytorch` [3].

The raw output of the neural network is a matrix $A \in \mathbb{R}^{m \times m}$ whose diagonal is set to be all zeros. Let $A_{i,:}$ and $A_{:,j}$ denote $A$'s $i^{\text{th}}$ row and $j^{\text{th}}$ column, respectively, and let $\sigma : \mathbb{R}^m \to (0,1)^m$ be the softmax function,

$$\sigma(x)_v = \frac{e^{\beta x_v}}{\sum_{j=1}^{m} e^{-\beta x_w}}. \tag{1}$$

Our experiments all use $\beta = 1$. In global synchrony experiments, the underlying undirected graph, $G$, had a fixed average weighted node degree of $\langle d \rangle = \frac{1}{m} \sum_{i,j} K_{i,j} = 1$. This was achieved by first row-normalizing $A$ by

$$A_{i,:} \leftarrow \langle d \rangle \sigma(A_{i,:}) \tag{2}$$

and then symmetrizing:

$$K = \frac{1}{2}\left(A + A^T\right). \tag{3}$$

The diagonal was then zeroed out to avoid nontrivial self-interactions in Case III. Note that $K$ is positive ($K_{ij} > 0$ for all $i, j$) so that all oscillator interactions are attractive. Brede [4, 5, 6] achieved the same effect by using link switching on an unweighted graph, which preserves $\langle d \rangle$ during optimization at the cost of foregoing differentiability.

In cluster synchrony experiments, there were no graph constraints of experimental interest, but $K$ was still normalized for stability of dynamics and to facilitate comparisons to control models. Specifically, $A$ was first row-normalized by

$$A_{i,:} \leftarrow \frac{A_{i,:}}{\|A_{i,:}\|_2} \tag{4}$$

and then symmetrized as in Eq. 3. Normalizing by the Euclidean norm permits negative interactions which are in fact necessary for strong cluster synchrony. Note also that $K$ itself is not row-normalized as a result of symmetrization, although the Frobenius norm of $K$ is upper-bounded.

### 1.3 Dynamics

Global synchrony experiments used the full Kuramoto dynamics with heterogeneous oscillators, namely

$$\dot{\theta}_i = \omega_i + \sum_{j=1}^{n} K_{ij} \sin(\theta_j(t - \tau_j) - \theta_i(t)) + b_i \sin(\theta_i). \tag{5}$$

In cluster synchrony experiments, heterogeneity was in fact the target state, so disorder in the system was removed, leaving a reduced dynamics on XY spins:

$$\dot{\theta}_i = \sum_{j=1}^{n} K_{ij} \sin(\theta_j(t) - \theta_i(t)). \tag{6}$$

In all cases, the dynamics were simulated using the `torchdiffeq` software package [7] on an NVIDIA Titan X GPU. Eq. 1 in the main text was solved with Euler's method with a step-size of $\alpha = .1$, but other solvers are also available in our coding framework. The simulation ran for 200 steps in the global synchrony experiments and the first 100 steps were used as a burn-in period. In the cluster synchrony experiments, transients were shorter since oscillators were homogeneous so we only used 100 steps with no burn-in.

For the large network setting used during evaluation, $n = N = 10,000$, the coupling matrix, $K$, was too large to hold in GPU memory. There are two options for reducing the memory load imposed by $K$: 1) solve a deterministic version of the dynamics with sparsified interactions, or 2) solve a stochastic version of the full interactions. The former route was taken, for instance, by [8] who used diffusive couplings to build an oscillator model of image segmentation. This makes sense for images, which have inherently local structure. Its utility is less clear for systems where global interaction (e.g., our global synchrony experiments) is at play.

We therefore opt for the second method by using a stochastic approximation to Euler's method in which only a uniformly random size-$m$ subset of oscillators was updated at every Euler step. We refer to $m$ as the "dynamic batch size" to distinguish it from the "mini-batch size", $n$, representing the size of the whole graph, which is, in turn, distinguished from the size, $N$, of the whole data set. In detail, we solve an initial value problem (IVP) defined by $\frac{dy}{dt} = f(y)$ for $y \in \mathbb{R}^n$ and $t \in \mathbb{R}$ such that $y(0) = y_0$. Let $a$ be vector in $\{0,1\}^n$ such that $\sum_i a_i = m$ and let $a_\sigma$ denote a random permutation of the elements of $a$. Let $\{Y_i\}_{i=1}^T$ be the sequence in $\mathbb{R}^n$ generated by the random updating scheme,

$$Y_{i+1} = Y_i + \alpha t(a_{\sigma_i} \bullet f(Y_i)), \tag{7}$$

where $\alpha = t_{i+1} - t_i$ for all $i$, $\sigma_i$ is a random sample from the uniform distribution on permutations $\Sigma \sim U([1, n!])$, and $\bullet$ denotes element-wise multiplication. Each $a_{\sigma_i}$ masks $m$ random dimensions of $Y_i$ so that only the other $n - m$ dimensions are updated at step $i$.

This stochastic updating scheme makes KuraNet completely size-agnostic, in the sense that, given infinite compute time, it can technically learn optimal dynamics on arbitrarily-sized networks. We do, however, incur a substantial cost: random updating makes the asymptotic error of the Euler update one polynomial degree worse. For instance, let:

$$p(t) = O(q(t)) \tag{8}$$

mean that $\limsup_{t\to 0} \frac{\|p(t)\|}{q(t)} < \infty$. With stochastic dynamics, what would be $O(\alpha^2)$ error after one update step in the deterministic scheme becomes $O(\alpha)$ (in expectation), and what would be $O(\alpha)$ after $i$ steps becomes $O(1)$ (again in expectation). This is encapsulated in the following proposition, whose proof is given in Section 1.5:

**Proposition 1** *(Expected truncation errors). Let $y(t) \in \mathbb{R}^n$ be a twice-differentiable function of $t \in \mathbb{R}$ obeying $\frac{dy}{dt} = f(y)$ and $y(0) = y_0$. Assume $f$ is differentiable and Lipschitz with constant L. Let $\{Y_i\}_{i\in\mathbb{N}}$ be the sequence generated by the updating scheme in Eq. 7. If $Y_i = y_i = y(t_i)$, then the expected local truncation error at step $t_{i+1}$, $ELTE(\alpha)$, is*

$$ELTE(\alpha) = O(\alpha). \tag{9}$$

*If $Y_0 = y(0)$, then the magnitude of the expected global truncation error at step $t_{i+1}$, $EGTE(\alpha)$, obeys*

$$EGTE(\alpha) = O(1). \tag{10}$$

Since we train in the small network regime, where $m = n$, this error does not affect learning. However, it does affect evaluation in the large-$n$ regime, making our results, especially for global synchrony experiments, very conservative. The exact amount of error incurred by random sampling can be controlled by increasing $m$.

### 1.4 Training and Testing

KuraNet was trained with the Adam optimizer [9] with learning rate $\eta = 5e-5$. Gradients were calculated by using the adjoint system solver in `torchdiffeq`. Following standard machine learning protocol, gradients were clipped to have euclidean norm at most 1.0 to improve the stability of learning. In each experiment, KuraNet was exposed to all data in the training set divided into mini-batches of size $n = 100$. Case I and Case II of the global synchrony experiments converged after 1 epoch and Case III took 3. We set the number of epochs to be 5 for the mixture distribution clustering experiments, though some (e.g. Moons, GMM2) converged much faster than this. Image segmentation took substantially longer to learn: most experiments converged within 25-40 epochs, but to allow for the possibility of slower converging but ultimately better performing models, we trained the system on 120 epochs.

Each model was evaluated according to three testing regimes according to what setting was novel: the node features, the network size, or both. In the first case (Data Testing), losses were measured individually on 100 mini-batches, each of size $n = 100$, from the test set and then averaged. In the second case (Size Testing), a single loss was measured on one network of size $n = N = 10,000$ whose nodes used data from the full *training set*. In the second case (Data+Size Testing), a single loss was measured on one network of size $n = N = 10,000$ whose nodes used data from the full *test set*. The latter two regimes used a dynamic batch size of $m = 100$ to accommodate the large network.

Additionally, models trained on BSDS were evaluated by the symmetric best dice metric [10], a common quality measure for image segmentation defined as follows. A segmentation of an image is a partition of pixels into a set of disjoint subsets $\mathcal{S} = \{S_i\}_{i=1}^p$ each of which has $|S_i|$ pixels. Consider two segmentations, $S^a$ and $S^b$, one of which we take to be the ground truth and the other we take to be a prediction. The *best dice score* of the prediction is

$$BD(S^a, S^b) = \frac{1}{p}\sum_{i=1}^{p} \max_{j \le j \le p} \frac{2|S_i^a \cap S_j^b|}{|S_i^b| + |S_j^b|}, \tag{11}$$

where $S^a$ has $p$ segments and $S^b$ has $q$ segments. The symmetric best dice score, $SBD(S^a, S^b)$ is then defined as the minimum of $BD(S^a, S^b)$ and $BD(S^b, S^a)$.

### 1.5 Proof of Proposition 1

We prove Eq. 9 first and then Eq. 10. Assuming $Y_i = y(t_i)$, the true value of $y$ at the next step can be expanded

$$\begin{aligned} y(t_{i+1}) &= y(t_i + \alpha) \\ &= y(t_i) + \alpha y'(t_i) + \frac{1}{2}\alpha^2 y''(t_i) + O(\alpha^3) \\ &= y(t_i) + \alpha f(y(t_i)) + \frac{1}{2}\alpha^2 y''(t_i) + O(\alpha^3), \end{aligned}$$

since $y$ is twice-differentiable. The local truncation error can then be computed as

$$\begin{aligned} \epsilon_i &= y(t_i + \alpha) - Y_{i+1} \\ &= y(t_i + \alpha) - Y_i - \alpha(a_{\sigma_i} \bullet f(Y_i)) \\ &= y(t_i + \alpha) - y(t_i) - \alpha(a_{\sigma_i} \bullet f(y(t_i))) \\ &= y(t_i) + \alpha f(y(t_i)) + \frac{1}{2}\alpha^2 y''(t_i) + O(\alpha^3) - y(t_i) - \alpha(a_{\sigma_i} \bullet f(y(t_i))) \\ &= \alpha f(y(t_i)) + \frac{1}{2}\alpha^2 y''(t_i) + O(\alpha^3) - \alpha(a_{\sigma_i} \bullet f(y(t_i))) \\ &= \alpha f(y(t_i)) \bullet (\mathbf{1} - a_{\sigma_i}) + \frac{1}{2}\alpha^2 y''(t_i) + O(\alpha^3), \end{aligned}$$

where the third line follows from $Y_i = y(t_i)$ and $\mathbf{1}$ is the vector of all ones. Consequently,

$$\begin{aligned} \|\epsilon_i\| &= \|\alpha f(y(t_i)) \bullet (\mathbf{1} - a_{\sigma_i}) + \frac{1}{2}\alpha^2 y''(t_i) + O(\alpha^3)\| \\ &\leq \|\alpha f(y(t_i)) \bullet (\mathbf{1} - a_{\sigma_i})\| + \frac{1}{2}\|\alpha^2 y''(t_i)\| + O(\alpha^3) \\ &\leq \alpha \|f(y(t_i))\| \|(\mathbf{1} - a_{\sigma_i})\| + \frac{1}{2}\alpha^2 \|y''(t_i)\| + O(\alpha^3) \end{aligned} \tag{12}$$

since $\|v \bullet w\| \leq \|v\|\|w\|$ for $v, w \in \mathbb{R}^n$. By the monotonicity and linearity of the expected value, we have

$$\begin{aligned} ELTE(\alpha) &= \mathbb{E}_\Sigma\left[\|\epsilon_i\|\right] \\ &\leq \alpha \|f(y(t_i))\| \, \mathbb{E}_\Sigma\left[\|(\mathbf{1} - a_{\sigma_i})\|\right] + \frac{1}{2}\alpha^2 \|y''(t_i)\| + O(\alpha^3) \end{aligned}$$

Note that only one term in this last line depends on the random variable $a_{\sigma_i}$ and that the expected value of $(\mathbf{1} - a_{\sigma_i})$ is the $n$-dimensional vector with $(1 - \frac{m}{n})$ for each element. It follows that

$$\begin{aligned} ELTE(\alpha) &\leq \alpha \left(1 - \frac{m}{n}\right) f(y(t_i)) + \frac{1}{2}\alpha^2 y''(t_i) + O(\alpha^3) \\ &= O(\alpha). \end{aligned} \tag{13}$$

We now turn to the proof of Eq. 10 and let $Y_0 = y(0)$. We note that, since $f$ is differentiable everywhere, $y''$ exists and is continuous. By the mean value theorem, there exists a $t_i^* \in (t_i - \alpha, t_i + \alpha)$ such that

$$y(t_i + \alpha) = y(t_i) + \alpha f(y_i) + \frac{1}{2}\alpha^2 y''(t_i^*). \tag{14}$$

Observe that the error after $i$ updates, $\epsilon_i$, follows the recurrence relation

$$\begin{aligned} \epsilon_{i+1} &= y_{i+1} - Y_{i+1} \\ &= y_i - Y_i + \alpha(f(y_i)) - \alpha_{\sigma_i} \bullet f(Y_i) + \frac{1}{2}\alpha^2 y''(t_i^*) \\ &= \epsilon_i + \alpha\left(f(y_i) - a_{\sigma_i} \bullet f(Y_i)\right) + \frac{1}{2}\alpha^2 y''(t_i^*) \end{aligned} \tag{15}$$

By repeatedly applying the triangle inequality and using the fact that $f$ is Lipschitz, we find that the magnitude of the global truncation error, $\|\epsilon_i\|$ obeys

$$\begin{aligned}
\|\epsilon_{i+1}\| &= \|\epsilon_i + \alpha\left(f(y_i) - a_{\sigma_i} \bullet f(Y_i)\right) + \frac{1}{2}\alpha^2 y''(t_i^*)\| \\
&\leq \|\epsilon_i\| + \|\alpha\left(f(y_i) - a_{\sigma_i} \bullet f(Y_i)\right)\| + \|\frac{1}{2}\alpha^2 y''(t_i^*)\| \\
&= \|\epsilon_i\| + \|\alpha\left(f(y_i) - f(Y_i) + f(Y_i) - a_{\sigma_i} \bullet f(Y_i)\right)\| + \|\frac{1}{2}\alpha^2 y''(t_i^*)\| \\
&\leq \|\epsilon_i\| + \alpha L\|y_i - Y_i\| + \alpha(\mathbf{1} - a_{\sigma_i}) \bullet \|f(Y_i)\| + \|\frac{1}{2}\alpha^2 y''(t_i^*)\| \\
&= \|(1+\alpha L)\epsilon_i\| + \alpha(\mathbf{1} - a_{\sigma_i}) \bullet \|f(Y_i)\| + \|\frac{1}{2}\alpha^2 y''(t_i^*)\|
\end{aligned}$$

almost surely. By the monotonicity of expected value, we can recast this inequality in expectation by

$$\begin{aligned}
\mathbb{E}_\Sigma\left[\|\epsilon_{i+1}\|\right] &\leq \mathbb{E}_\Sigma\left[\|(1+\alpha L)\epsilon_i\|\right] + \alpha\,\mathbb{E}_\Sigma\left[(\mathbf{1} - a_{\sigma_i}) \bullet \|f(Y_i)\|\right] + \|\frac{1}{2}\alpha^2 y''(t_i^*)\| \\
&= (1+\alpha L)\,\mathbb{E}_\Sigma\left[\|\epsilon_i\|\right] + \alpha(1 - \frac{m}{n})\|f(Y_i)\| + \|\frac{1}{2}\alpha^2 y''(t_i^*)\|
\end{aligned}$$

Since $f$ is continuous and Lipschitz it has bounded first derivative and consequently both $f$ and

$$y''(t) = \frac{df}{dy} f$$

are bounded. Hence, there exist $D_1, D_2 > 0$ such that

$$\begin{aligned}
\mathbb{E}_\Sigma\left[\|\epsilon_{i+1}\|\right] &\leq (1+\alpha L)\,\mathbb{E}_\Sigma\left[\|\epsilon_i\|\right] + \alpha(1 - \frac{m}{n})D_1 + \frac{1}{2}\alpha^2 D_2 \\
&:= w_{i+1}
\end{aligned} \tag{16}$$

Thus, $\{w_i\}$ is a sequence satisfying $\mathbb{E}_\Sigma[\|\epsilon_i\|] \leq w_i$ and

$$w_{i+1} = (1+\alpha L)w_i + b, \tag{17}$$

where $b = \alpha(1 - \frac{m}{n})D_1 + \frac{1}{2}\alpha^2 D_2$. A solution to Eq. 17 has the form

$$w_i = c_i \bar{w}_i, \tag{18}$$

where $\bar{w}_i$ is the solution to the homogeneous equation

$$\bar{w}_{i+1} = (1+\alpha L)\bar{w}_i$$

and $c_i$ is a constant with $c_0 = 0$. We can verify that the homogeneous equation has solution

$$\bar{w}_i = (1+\alpha L)^i.$$

Substituting the solution Eq. 18 into Eq. 17 and using the homogeneous solution gives

$$\begin{aligned}
c_{i+1}(1+\alpha L)^{i+1} &= (1+\alpha L)w_i + b \\
&= (1+\alpha L)c_i\bar{w}_i + b \\
&= c_i(1+\alpha L)^{i+1} + b,
\end{aligned}$$

so that $c_{i+1} = c_i + \frac{b}{(1+\alpha L)^{i+1}}$. Recursively substituting for $c_i$ yields the geometric series

$$\begin{aligned}
c_{i+1} &= b\sum_{\ell=1}^{i+1} \frac{1}{(1+\alpha L)^\ell} \\
&= \frac{b}{1+\alpha L}\frac{1 - \frac{1}{(1+\alpha L)^{i+1}}}{1 - \frac{1}{1+\alpha L}} \\
&= \frac{b}{\alpha L}\left(1 - \frac{1}{(1+\alpha L)^{i+1}}\right) \\
&= \frac{(1-\frac{m}{n})D_1 + \frac{1}{2}\alpha D_2}{L}\left(1 - \frac{1}{(1+\alpha L)^{i+1}}\right)
\end{aligned} \tag{19}$$

We can now substitute this value of $c_{i+1}$ into Eqs. 17 and 18:

$$\begin{aligned} w_{i+1} &= c_{i+1}\bar{w}_{i+1} \\ &= c_{i+1}(1+\alpha L)^{i+1} \\ &= \left((1-\frac{m}{n})\frac{D_1}{L} + \frac{1}{2L}\alpha D_2\right)\left(1 - \frac{1}{(1+\alpha L)^{i+1}}\right)(1+\alpha L)^{i+1} \\ &= \left((1-\frac{m}{n})\frac{D_1}{L} + \frac{1}{2L}\alpha D_2\right)\left((1+\alpha L)^{i+1} - 1\right) \end{aligned} \tag{20}$$

Finally, we note that

$$\begin{aligned} \lim_{\alpha\to 0}(1+\alpha L)^{i+1} &= \lim_{\alpha \to 0}(1+\alpha L)^{(t_{i+1}-t_0)/\alpha} \\ &= e^{L(t_{i+1}-t_0)}. \end{aligned}$$

Hence, when $\alpha$ is small, we can approximate Eq. 20 by

$$\begin{aligned} w_{i+1} &= \left((1-\frac{m}{n})\frac{D_1}{L} + \frac{1}{2L}\alpha D_2\right)\left((1+\alpha L)^{i+1} - 1\right) \\ &\approx \left((1-\frac{m}{n})\frac{D_1}{L} + \frac{1}{2L}\alpha D_2\right)\left(e^{L(t_{i+1}-t_0)} - 1\right) \\ &= O(1) \end{aligned} \tag{21}$$

so that $\|\epsilon_{i+1}\| \leq w_i = O(1)$, as desired.

## 2 Detailed Clustering Results

### 2.1 Mixture Distributions

The value of the cluster synchrony loss (Eq. 5, main text) measured at the last time step during dynamics in various testing regimes is displayed in Table 1. As in the main text, the three testing regimes correspond to which between the node features (Data) and network size (Size) was generalized (including both, Data + Size). Parenthetical values are a randomized control model whose couplings are normalized in the same way as the optimized model.

Performance of the optimized system is favorable in all cases, though it is difficult to extract any principle about which settings are easier or harder, except that the large network regime typically results in lower losses. The approximation to the thermodynamic limit in this regime likely helps filter out the undue influence of a few bad couplings sometimes observed for smaller systems. The two-cluster cases (Moons, Circles, Spirals, GMM2) are generally easier with the exception of Spirals which is particularly tricky to separate when the arms of the spiral are tightly twisted (Fig. 1, upper right). Note that an increasing number of clusters does not necessarily result in a higher baseline control loss. While intra-group synchrony is typically harder with more clusters, this can result in a lower desynchrony loss. The final state of one simulation ($n = 100$) for each data set is depicted in Figure 1.

Training loss curves for each of 100 batches over the five epochs are shown in Figure 2. Curves are from the best seed out of ten. Note that the classes in GMM2 are linearly separable so the model learns to cluster the data essentially after one gradient descent step. A decrease in loss during training was often preceded by a long burn-in time. Seeds with a long burn-in during learning were typically worse than those with short ones, so they are not represented in any great numbers in Figure 2, except, for example, in GMM4. We note informally that the ease of escaping this burn-in regime for a data set with $k$ classes seems related number of integer divisors of $k$, with a larger number of divisors hindering learning and smaller number promoting it. We have not tested this observation, though it makes intuitive sense that the number of spurious clusterings is related to the number of factors of $k$.

The structure of couplings is depicted in Figures 3 and 4. The first figure shows couplings sorted by group belonging on a network of $n = 1000$ nodes. Figures 3 shows how the system learns a combined strategy of block and diffusive couplings: couplings between groups only depend on the group index and couplings grow weaker and more negative as the features grow more distant in the plane (note: GMM$k$ ground truth groups are indexed counterclockwise, with the first group closest 3 o'clock). This results in the off-diagonal positive couplings visible starting in $GMMk$ for $k \geq 4$. Another way to view this combined block-diffusive coupling is shown in Figure 4 where each panel depicts the relationship between couplings, $K_{ij}$, and the Euclidean distance between the node features $x^{(i)}$ and $x^{(j)}$. Data were taken from 10 networks each of size $n = 1000$. Couplings are colored blue when they connect two units within a group

and red when they connect two units in different groups. In general, intra-group couplings are strong and positive, and inter-group couplings are increasingly negative with $\|x^{(i)} - x^{(j)}\|_2$. The non-GMM$k$ are mild exceptions to this rule, having substantial negative intra-group couplings.

It is easy to visually evaluate the quality of clustering by examining the local mean fields in each group at the end of the dynamics (Figure 5). In each circular plot, we show the order parameter related to each ground truth group in the form of an arrow whose length is the mean field magnitude and whose angle is the mean field angle. The phase of each oscillator is shown in small dots around the circumference of the unit circle. Colors correspond to ground truth classes. In all cases, clusters are splay, as intended. This is the case for neither random models nor simple control models as the kind described in the main text, the latter of which can easily desynchronize two-cluster data but struggles with more groups.

### 2.2 Natural image segmentation

The results for natural images were much the same as in the simple mixture distribution case. The last eight rows of Table 1 contain numerical results for each image, indexed by the BSDS ID. An extended version of Fig. 4 in the main text is given in Fig. 6. Note once again that these images represent the combined training and testing set, while the data in Table 1 is only for the testing regimes. The images were quite large ($\sim 150,000$ pixels) and so we ran the dynamics for a very long time (1M Euler steps) using a dynamic batch size of $m = 100$. Note that the control values are quite a bit worse than those in the mixture distribution case, owing largely to the size of the networks at play.

Table 1: Cluster synchrony test results

| Dist. | Data | Size | Data + Size |
|---|---|---|---|
| Moons | 0.0029 (0.2789) | 0.0038 (0.5592) | 0.0032 (0.5594) |
| Circles | 0.0002 (0.5038) | 0.0.0000 (0.5025) | 0.0000 (0.5023) |
| Spirals | 0.0267 (0.4506) | 0.0190 (0.9262) | 0.0208 (0.4808) |
| GMM2 | 0.0000 (0.5000) | 0.0000 (0.5000) | 0.0000 (0.5000) |
| GMM3 | 0.0110 (0.2651) | 0.0044 (0.4472) | 0.0058 (0.4405) |
| GMM4 | 0.0500 (0.7142) | 0.0290 (0.7143) | 0.0286 (0.7143) |
| GMM5 | 0.0078 (0.2552) | 0.0024 (0.3919) | 0.0028 (0.3555) |
| GMM6 | 0.0088 (0.6612) | 0.0024 (0.7892) | 0.0023 (0.7992) |
| GMM7 | 0.0130 (0.8265) | 0.0055 (0.8265) | 0.0076 (0.8265) |
| GMM8 | 0.0164 (0.8344) | 0.0092 (0.8527) | 0.0089 (0.8531) |
| GMM9 | 0.0074 (0.2135) | 0.0028 (0.2180) | 0.0023 (0.2164) |
| GMM10 | 0.0151 (0.1439) | 0.0060 (0.1414) | 0.0075 (0.1343) |
| 118020 | 0.0137 (0.8022) | 0.0060 (0.8522) | 0.0060 (0.8521) |
| 124084 | 0.0237 (0.6763) | 0.0074 (0.8488) | 0.0079 (0.8494) |
| 189011 | 0.0493 (0.7410) | 0.0103 (0.8286) | 0.0107 (0.8277) |
| 229036 | 0.0502 (0.7617) | 0.0085 (0.8285) | 0.0089 (0.8284) |
| 247003 | 0.0496 (0.7574) | 0.0113 (0.8273) | 0.0117 (0.8261) |
| 296028 | 0.0228 (0.7403) | 0.0062 (0.8587) | 0.0063 (0.8578) |
| 317080 | 0.0509 (0.7601) | 0.0099 (0.8231) | 0.0090 (0.8227) |
| 361010 | 0.0404 (0.7326) | 0.0113 (0.8235) | 0.0125 (0.8240) |

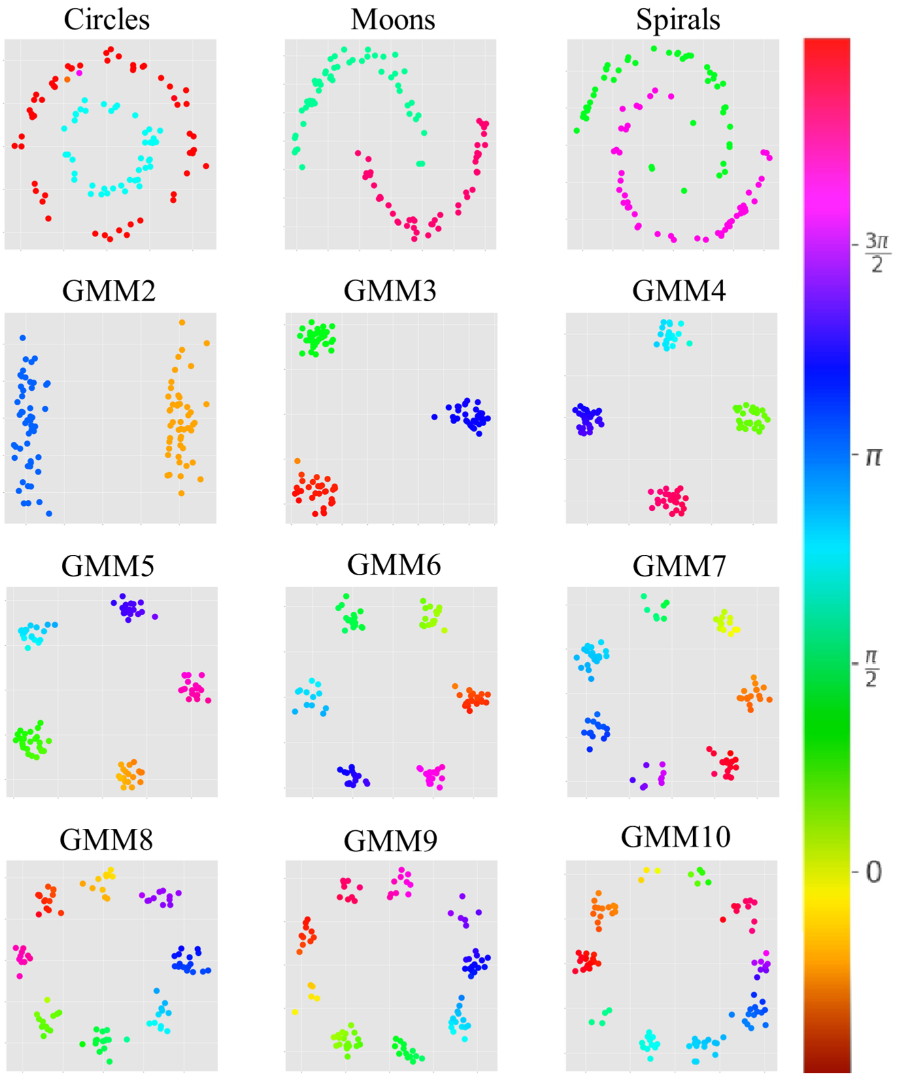


Figure 1: Final state of dynamics with $n = 100$ oscillators for each mixture distribution.

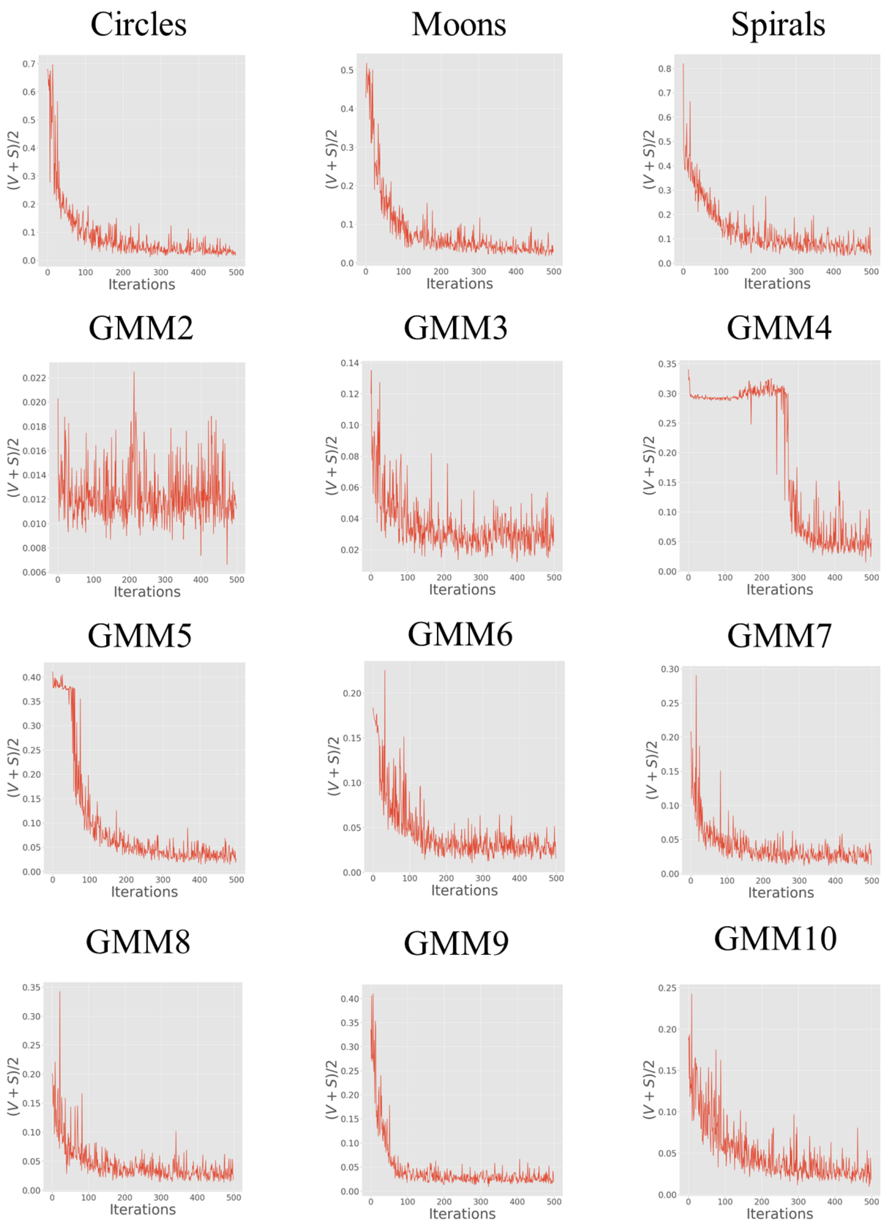


Figure 2: Training loss for each mixture distribution.

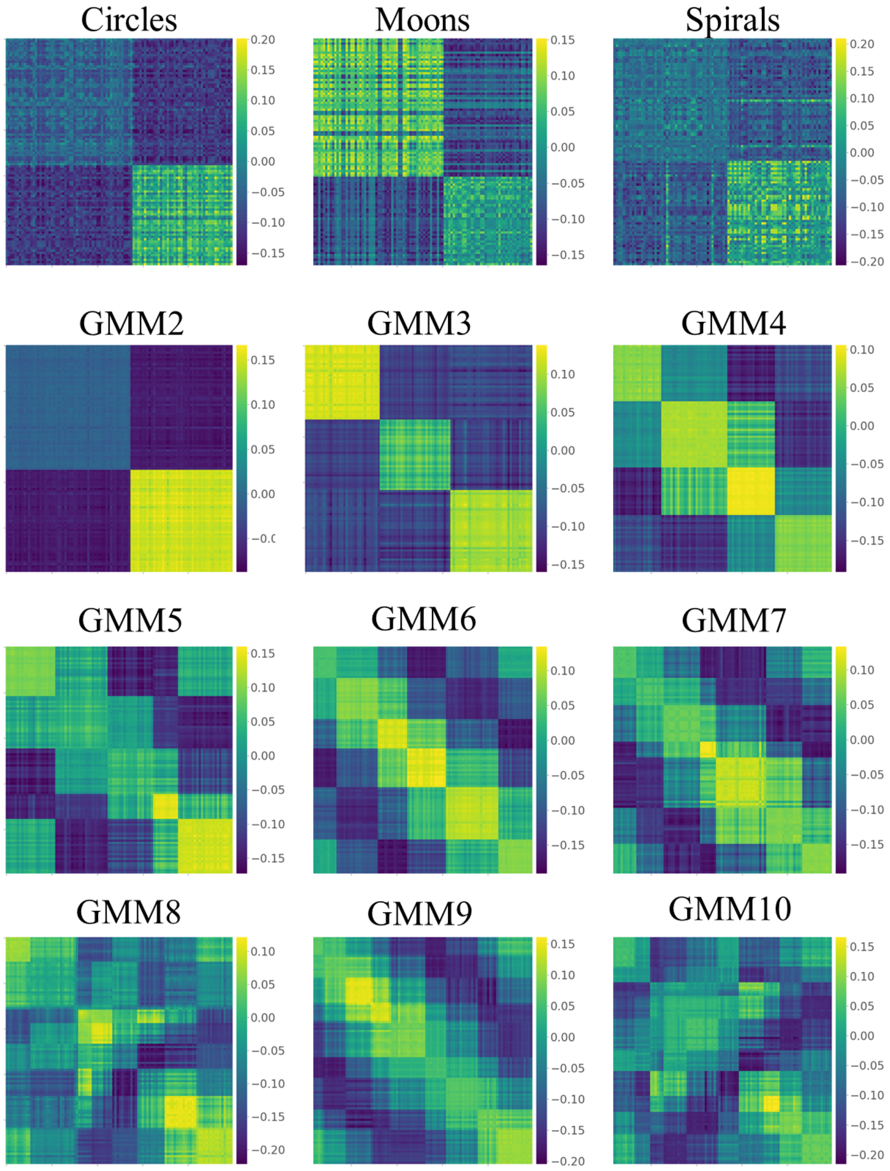


Figure 3: Couplings sorted by group belonging for $n = 1000$ oscillators and each mixture distribution.

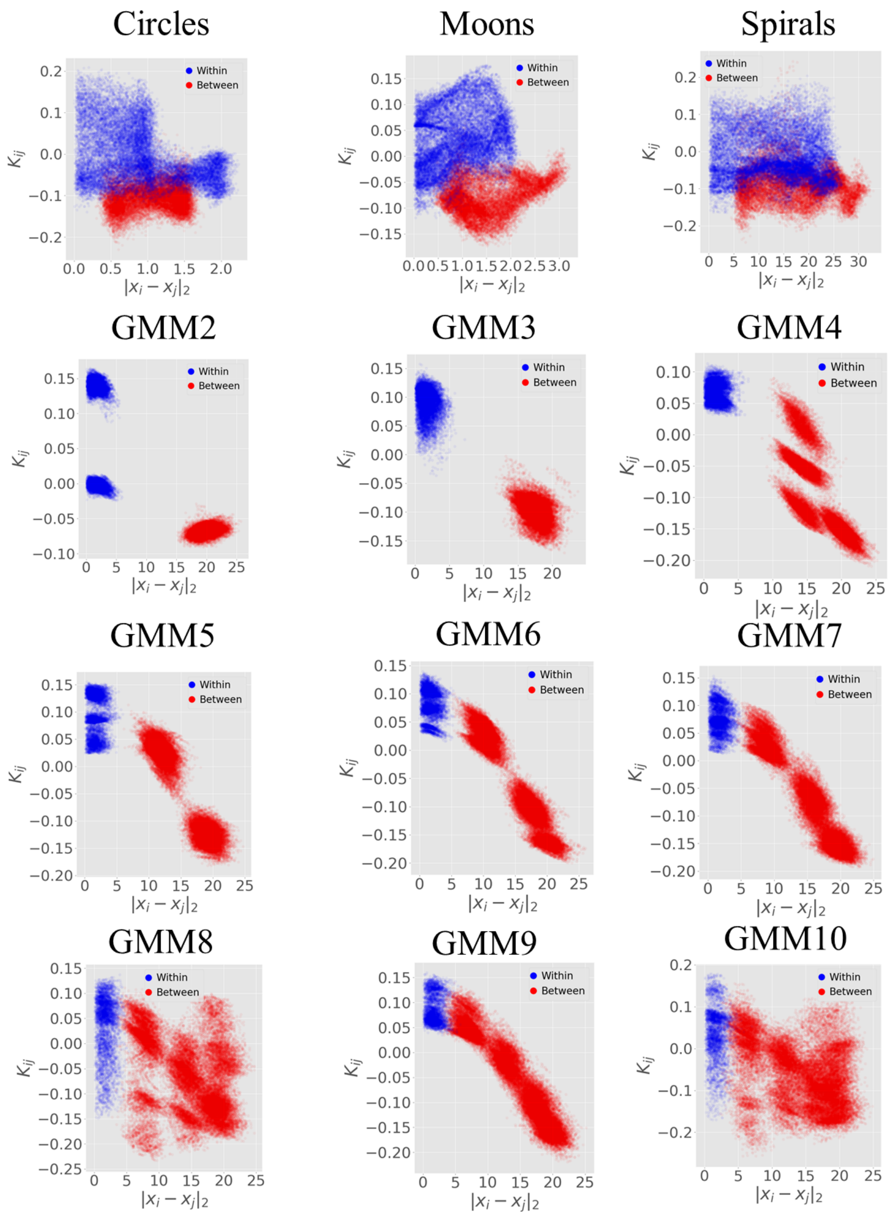


Figure 4: Relationship between couplings and Euclidean distance between node features collected from 10 networks of size $n = 1000$ for each mixture distribution.

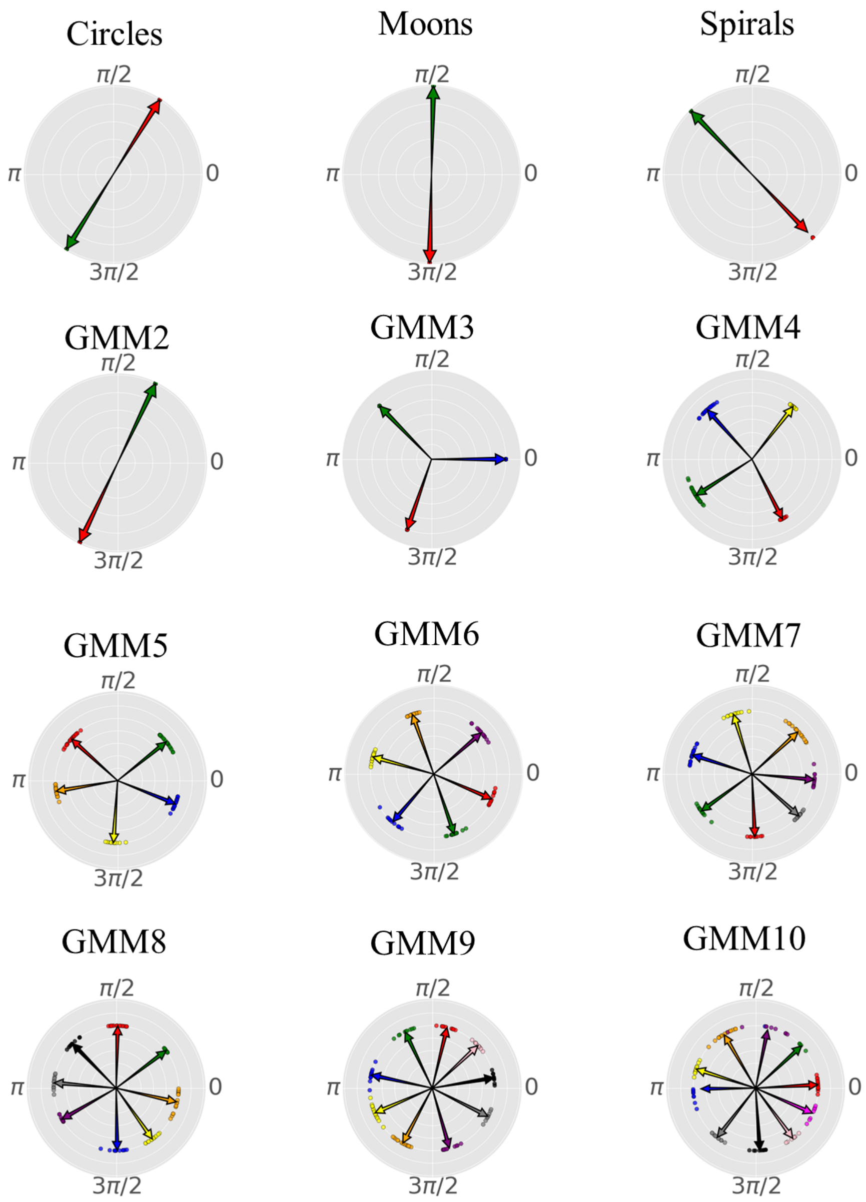


Figure 5: Local mean fields for each ground truth cluster for each mixture distribution. Colors denote true groups, not phase.

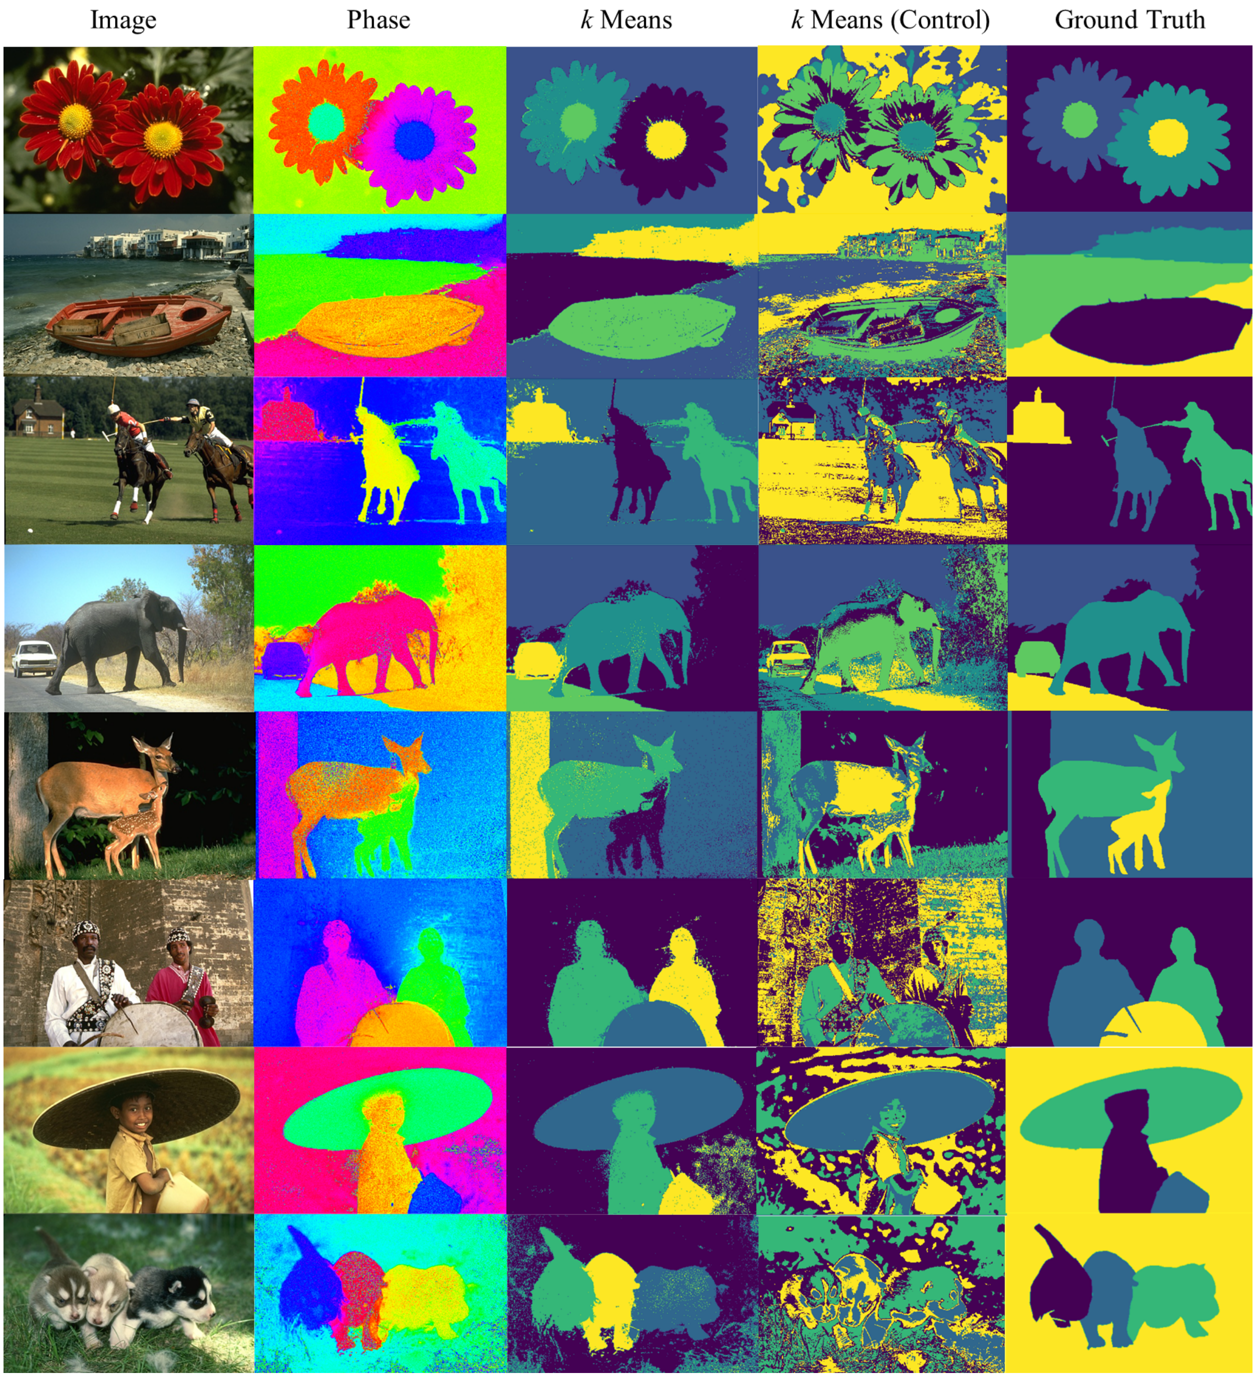


Figure 6: All image segmentation results.

## References

[1] Sergey Ioffe and Christian Szegedy. Batch Normalization : Accelerating Deep Network Training by Reducing Internal Covariate Shift. In *ICML'15: Proceedings of the 32nd International Conference on Machine Learning*, pages 448–456, Lille, France, 2015. Proceedings of Machine Learning Research.

[2] Adam Santoro, David Raposo, David G Barrett, Mateusz Malinowski, Razvan Pascanu, Peter Battaglia, and Timothy Lillicrap. A simple neural network module for relational reasoning. In I. Guyon, U. V. Luxburg, S. Bengio, H. Wallach, R. Fergus, S. Vishwanathan, and R. Garnett, editors, *Advances in Neural Information Processing Systems*, volume 30. Curran Associates, Inc., 2017.

[3] Adam Paszke, Sam Gross, Francisco Massa, Adam Lerer, James Bradbury, Gregory Chanan, Trevor Killeen, Zeming Lin, Natalia Gimelshein, Luca Antiga, Alban Desmaison, Andreas Kopf, Edward Yang, Zachary DeVito, Martin Raison, Alykhan Tejani, Sasank Chilamkurthy, Benoit Steiner, Lu Fang, Junjie Bai, and Soumith Chintala. Pytorch: An imperative style, high-performance deep learning library. In H. Wallach, H. Larochelle, A. Beygelzimer, F. d'Alché-Buc, E. Fox, and R. Garnett, editors, *Advances in Neural Information Processing Systems 32*, pages 8024–8035. Curran Associates, Inc., 2019.

[4] Markus Brede. Synchrony-optimized networks of non-identical Kuramoto oscillators. *Physics Letters, Section A: General, Atomic and Solid State Physics*, 372(15):2618–2622, 2008.

[5] M. Brede. Locals vs. global synchronization in networks of non-identical Kuramoto oscillators. *European Physical Journal B*, 62(1):87–94, 2008.

[6] Markus Brede. Construction principles for highly synchronizable sparse directed networks. *Physics Letters, Section A: General, Atomic and Solid State Physics*, 372(32):5305–5308, 2008.

[7] Ricky T.Q. Chen, Yulia Rubanova, Jesse Bettencourt, and David Duvenaud. Neural Ordinary Differential Equations. In *32nd Conference on Neural Information Processing Systems (NeurIPS 2018)*, Montréal, Canada, 2018. Curran Associates.

[8] Guoshen Yu and Jean Jacques Slotine. Visual grouping by neural oscillator networks. *IEEE Transactions on Neural Networks*, 20(12):1871–1884, 2009.

[9] Diederik P. Kingma and Jimmy Ba. Adam: A method for stochastic optimization, 2017.

[10] Hanno Scharr, Massimo Minervini, Andrew P. French, Christian Klukas, David M. Kramer, Xiaoming Liu, Imanol Luengo, Jean Michel Pape, Gerrit Polder, Danijela Vukadinovic, Xi Yin, and Sotirios A. Tsaftaris. Leaf segmentation in plant phenotyping: a collation study. *Machine Vision and Applications*, 27(4):585–606, 2016.
